# Supplementary material for: Current state and prospects of R-packages for the design of experiments
Source: arXiv:2206.07532 ancillary file (2022-12-14)
Supplement: Supplementary file 1 [file supp.pdf]

# Supplementary material for "Current status and prospects of R-packages for the design of experiments"

Emi Tanaka Dewi Amaliah

Table S1: A summary table for the CRAN task view that shows in order: the name of the task view, the full topic name, the total of packages, the total number of contributors, the average number of contributors, and the intra-connectivity. The intra-connectivity measures the percentage of packages that depends, suggest or imports at least one other package within the same task view. A low intra-connectivity suggests that development within the topic mostly occur in silos whilst high intra-connectivity suggests that there are more interactions within the topic. The row is ordered by the average number of contributors.

| Name | Topic | # of packages | Total # of contributors | Average # of contributors | Intra-connectivity (%) |
|---|---|---|---|---|---|
| ExperimentalDesign | Design of Experiments (DoE) & Analysis of Experimental Data | 112 | 211 | 2.27 | 29 |
| SportsAnalytics | Sports Analytics | 78 | 149 | 2.32 | 17 |
| MedicalImaging | Medical Image Analysis | 32 | 53 | 2.44 | 44 |
| MetaAnalysis | Meta-Analysis | 157 | 351 | 2.63 | 43 |
| ChemPhys | Chemometrics and Computational Physics | 75 | 162 | 2.65 | 28 |
| ClinicalTrials | Clinical Trial Design, Monitoring, and Analysis | 59 | 141 | 2.76 | 31 |
| Distributions | Probability Distributions | 257 | 597 | 2.88 | 45 |
| Survival | Survival Analysis | 239 | 558 | 2.92 | 73 |
| ExtremeValue | Extreme Value Analysis | 37 | 89 | 2.95 | 41 |
| Optimization | Optimization and Mathematical Programming | 136 | 328 | 3.04 | 29 |
| TimeSeries | Time Series Analysis | 339 | 793 | 3.04 | 58 |
| OfficialStatistics | Official Statistics & Survey Statistics | 131 | 325 | 3.06 | 40 |
| Hydrology | Hydrological Data and Modeling | 100 | 252 | 3.09 | 24 |
| NumericalMathematics | Numerical Mathematics | 115 | 271 | 3.14 | 63 |
| Databases | Databases with R | 43 | 95 | 3.23 | 77 |

*(Continued on next page...)*

Table S1: A summary table for the CRAN task view that shows in order: the name of the task view, the full topic name, the total of packages, the total number of contributors, the average number of contributors, and the intra-connectivity. The intra-connectivity measures the percentage of packages that depends, suggest or imports at least one other package within the same task view. A low intra-connectivity suggests that development within the topic mostly occur in silos whilst high intra-connectivity suggests that there are more interactions within the topic. The row is ordered by the average number of contributors. *(continued)*

| Name | Topic | # of packages | Total # of contributors | Average # of contributors | Intra-connectivity (%) |
|---|---|---|---|---|---|
| WebTechnologies | Web Technologies and Services | 201 | 428 | 3.25 | 90 |
| NaturalLanguageProcessing | Natural Language Processing | 56 | 130 | 3.30 | 62 |
| Bayesian | Bayesian Inference | 213 | 621 | 3.35 | 49 |
| FunctionalData | Functional Data Analysis | 40 | 109 | 3.38 | 60 |
| Robust | Robust Statistical Methods | 59 | 136 | 3.41 | 75 |
| Psychometrics | Psychometric Models and Methods | 230 | 567 | 3.41 | 69 |
| Tracking | Processing and Analysis of Tracking Data | 46 | 149 | 3.46 | 48 |
| Cluster | Cluster Analysis & Finite Mixture Models | 108 | 305 | 3.47 | 39 |
| Econometrics | Econometrics | 152 | 363 | 3.50 | 81 |
| Finance | Empirical Finance | 158 | 426 | 3.61 | 57 |
| MissingData | Missing Data | 210 | 740 | 3.99 | 42 |
| SpatioTemporal | Handling and Analyzing Spatio-Temporal Data | 81 | 269 | 4.04 | 70 |
| Spatial | Analysis of Spatial Data | 197 | 618 | 4.26 | 83 |
| GraphicalModels | Graphical Models | 32 | 109 | 4.38 | 78 |
| Pharmacokinetics | Analysis of Pharmacokinetic Data | 29 | 109 | 4.55 | 21 |
| HighPerformanceComputing | High-Performance and Parallel Computing with R | 83 | 315 | 4.75 | 63 |
| DifferentialEquations | Differential Equations | 27 | 114 | 4.96 | 56 |
| Environmetrics | Analysis of Ecological and Environmental Data | 93 | 383 | 5.02 | 74 |
| MachineLearning | Machine Learning & Statistical Learning | 102 | 488 | 5.63 | 50 |
| TeachingStatistics | Teaching Statistics | 46 | 236 | 6.35 | 57 |
| ReproducibleResearch | Reproducible Research | 102 | 524 | 6.49 | 76 |
| ModelDeployment | Model Deployment with R | 31 | 146 | 6.55 | 74 |

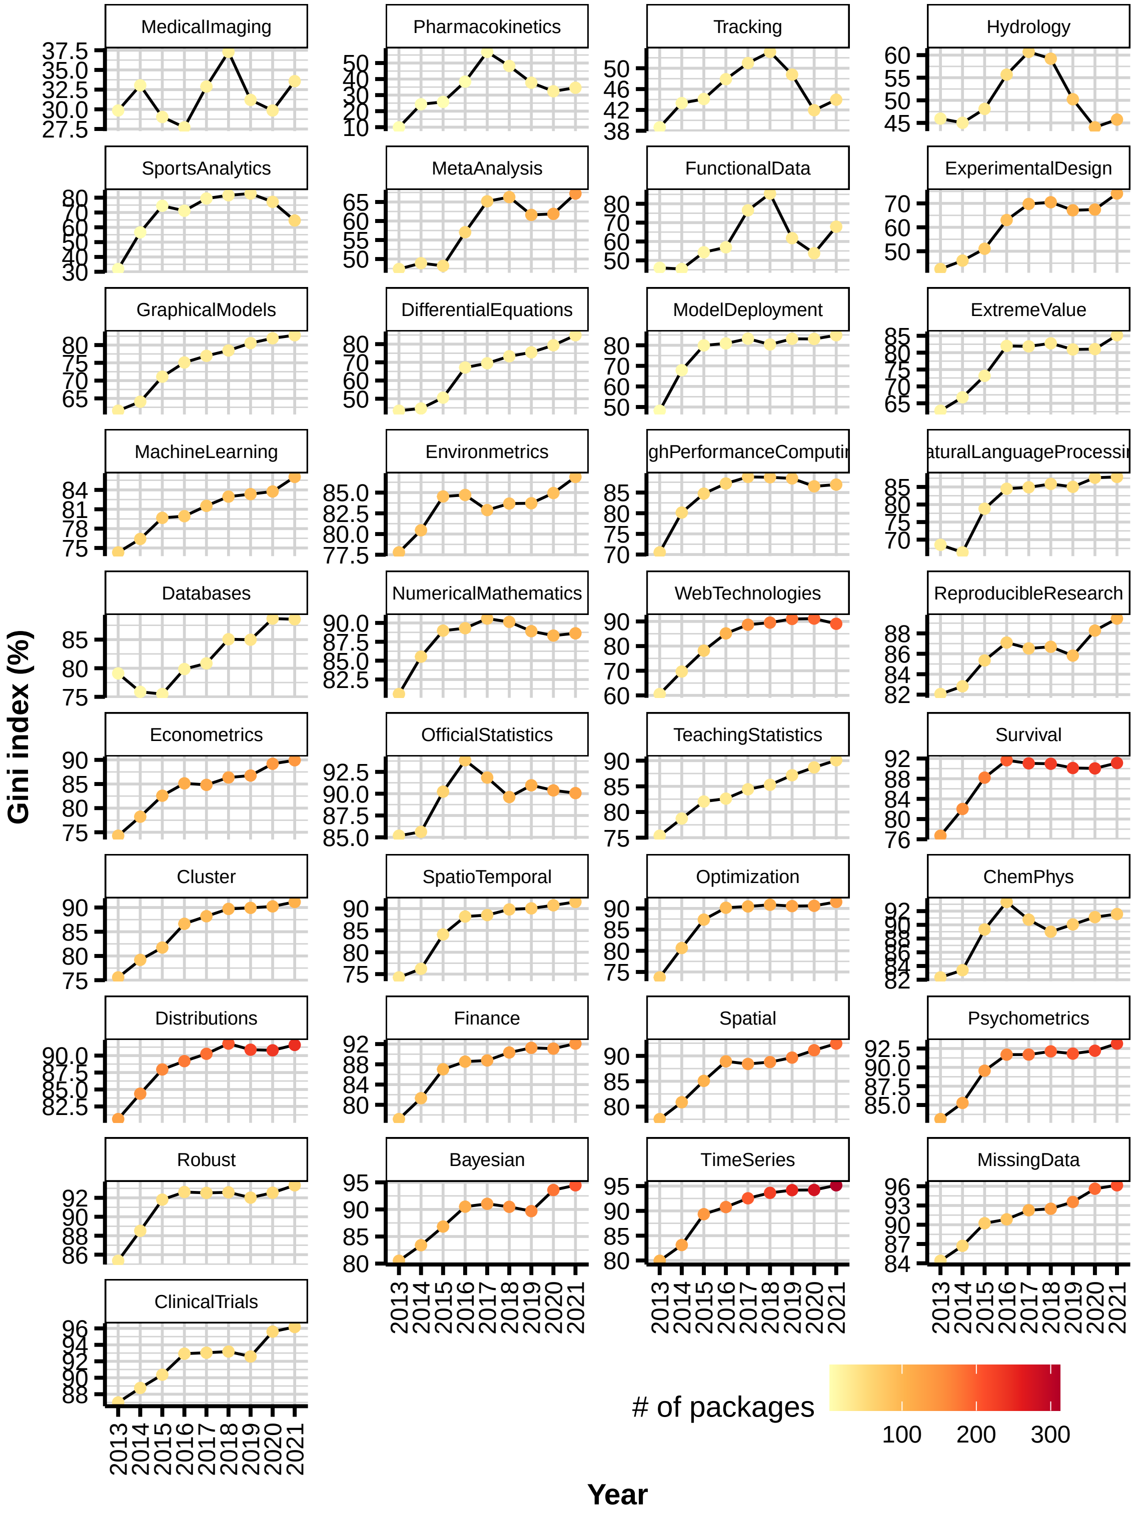


Figure S1: The points show the Gini index of the download counts by year facetted by CRAN task view with the color showing the number of packages. The grey line shows the distribution of the Gini index across years for all other CRAN task views. The facets are ordered by increasing value of the Gini index in 2021.

# Session information

**R version 4.1.2 (2021-11-01)**

**Platform:** x86_64-apple-darwin17.0 (64-bit)

**locale:** en_AU.UTF-8||en_AU.UTF-8||en_AU.UTF-8||C||en_AU.UTF-8||en_AU.UTF-8

**attached base packages:**

**other attached packages:**

- AsioHeaders(v.1.16.1-1)
- BH(v.1.75.0-0)
- DBI(v.1.1.1)
- DT(v.0.23)
- MASS(v.7.3-54)
- Matrix(v.1.3-4)
- R6(v.2.5.1)
- RColorBrewer(v.1.1-2)
- Rcpp(v.1.0.8)
- RcppArmadillo(v.0.10.8.1.0)
- RcppEigen(v.0.3.3.9.1)
- SnowballC(v.0.7.0)
- V8(v.4.2.0)
- anytime(v.0.3.9)
- askpass(v.1.1)
- assertthat(v.0.2.1)
- backports(v.1.3.0)
- base64enc(v.0.1-3)
- base64url(v.1.4)
- beeswarm(v.0.4.0)
- bit(v.4.0.4)
- bit64(v.4.0.5)
- blob(v.1.2.2)
- bookdown(v.0.24)
- broom(v.0.8.0)
- bslib(v.0.3.1)
- cachem(v.1.0.6)
- callr(v.3.7.0)
- cellranger(v.1.1.0)
- cli(v.3.3.0)
- clipr(v.0.7.1)
- coda(v.0.19-4)
- codetools(v.0.2-18)
- colorspace(v.2.0-2)
- commonmark(v.1.7)
- cpp11(v.0.4.2)
- cranlogs(v.2.1.1)
- crayon(v.1.4.2)
- crosstalk(v.1.2.0)
- ctv(v.0.9-2)
- curl(v.4.3.2)
- data.table(v.1.14.2)

- dbplyr(v.2.1.1)
- digest(v.0.6.29)
- distributional(v.0.2.2)
- dplyr(v.1.0.9)
- dtplyr(v.1.1.0)
- ellipsis(v.0.3.2)
- evaluate(v.0.14)
- fable(v.0.3.1)
- fabletools(v.0.3.1)
- fansi(v.1.0.2)
- farver(v.2.1.0)
- fastmap(v.1.1.0)
- feasts(v.0.2.2)
- fontawesome(v.0.2.2)
- forcats(v.0.5.1)
- fs(v.1.5.2)
- gargle(v.1.2.0)
- generics(v.0.1.2)
- ggbeeswarm(v.0.6.0)
- ggforce(v.0.3.3)
- ggnetwork(v.0.5.10)
- ggnewscale(v.0.4.5)
- ggplot2(v.3.3.5)
- ggraph(v.2.0.5)
- ggrepel(v.0.9.1)
- ggwordcloud(v.0.5.0)
- glue(v.1.6.1)
- googledrive(v.2.0.0)
- googlesheets4(v.1.0.0)
- graphlayouts(v.0.8.0)
- gridExtra(v.2.3)
- gtable(v.0.3.0)
- haven(v.2.4.3)
- here(v.1.0.1)
- highr(v.0.9)
- hms(v.1.1.1)
- htmltools(v.0.5.2)
- htmlwidgets(v.1.5.4)
- httpuv(v.1.6.3)
- httr(v.1.4.2)
- hunspell(v.3.0.1)
- ids(v.1.0.1)
- igraph(v.1.2.11)
- ineq(v.0.2-13)
- isoband(v.0.2.5)
- janeaustenr(v.0.1.5)
- jquerylib(v.0.1.4)
- jsonlite(v.1.7.3)
- kableExtra(v.1.3.4)
- knitr(v.1.37)
- labeling(v.0.4.2)

- later(v.1.3.0)
- lattice(v.0.20-45)
- lazyeval(v.0.2.2)
- lifecycle(v.1.0.1)
- lubridate(v.1.8.0)
- magrittr(v.2.0.2)
- mgcv(v.1.8-38)
- mime(v.0.12)
- modelr(v.0.1.8)
- munsell(v.0.5.0)
- network(v.1.17.2)
- networkD3(v.0.4)
- nlme(v.3.1-153)
- numDeriv(v.2016.8-1.1)
- openssl(v.2.0.2)
- pacman(v.0.5.1)
- pagedown(v.0.16)
- pander(v.0.6.6)
- parsedate(v.1.3.0)
- patchwork(v.1.1.1)
- pillar(v.1.7.0)
- pkgconfig(v.2.0.3)
- pkgsearch(v.3.1.0)
- plotly(v.4.10.0)
- pluralize(v.0.2.0)
- plyr(v.1.8.6)
- png(v.0.1-7)
- polyclip(v.1.10-0)
- prettyunits(v.1.1.1)
- processx(v.3.5.2)
- progress(v.1.2.2)
- progressr(v.0.9.0)
- promises(v.1.2.0.1)
- ps(v.1.6.0)
- purrr(v.0.3.4)
- qdapRegex(v.0.7.5)
- rappdirs(v.0.3.3)
- readr(v.2.1.2)
- readxl(v.1.3.1)
- rematch(v.1.0.1)
- rematch2(v.2.1.2)
- remotes(v.2.4.2)
- renv(v.0.15.5)
- reprex(v.2.0.1)
- reshape(v.0.8.8)
- rlang(v.1.0.2)
- rmarkdown(v.2.11)
- rprojroot(v.2.0.2)
- rstudioapi(v.0.13)
- rticles(v.0.22)
- rvest(v.1.0.2)

- sass(v.0.4.0)
- scales(v.1.1.1)
- selectr(v.0.4-2)
- servr(v.0.24)
- shiny(v.1.7.1)
- slider(v.0.2.2)
- sna(v.2.7)
- sourcetools(v.0.1.7)
- splitstackshape(v.1.4.8)
- statnet.common(v.4.6.0)
- stringi(v.1.7.6)
- stringr(v.1.4.0)
- svglite(v.2.0.0)
- sys(v.3.4)
- systemfonts(v.1.0.3)
- tarchetypes(v.0.6.0)
- targets(v.0.12.0)
- tibble(v.3.1.6)
- tidygraph(v.1.2.0)
- tidyr(v.1.2.0)
- tidyselect(v.1.1.2)
- tidytext(v.0.3.2)
- tidyverse(v.1.3.1)
- tinytex(v.0.36)
- tokenizers(v.0.2.1)
- tsibble(v.1.1.0)
- tweenr(v.1.0.2)
- tzdb(v.0.2.0)
- utf8(v.1.2.2)
- uuid(v.1.0-3)
- vctrs(v.0.4.1)
- vipor(v.0.4.5)
- viridis(v.0.6.2)
- viridisLite(v.0.4.0)
- visNetwork(v.2.1.0)
- vroom(v.1.5.7)
- warp(v.0.2.0)
- webshot(v.0.5.2)
- websocket(v.1.4.1)
- withr(v.2.4.3)
- xfun(v.0.29)
- xml2(v.1.3.2)
- xtable(v.1.8-4)
- yaml(v.2.2.2)

**loaded via a namespace (and not attached):**

- utils(v.4.1.2)
- tools(v.4.1.2)
- compiler(v.4.1.2)
- datasets(v.4.1.2)
- base(v.4.1.2)

- grDevices(v.4.1.2)
- grid(v.4.1.2)
- methods(v.4.1.2)
- graphics(v.4.1.2)
- stats(v.4.1.2)
